# Supplementary material for: Utilizing Synthetic Data in Supervised Learning for Robust 5-DoF Magnetic Marker Localization
Source: arXiv:2211.07556 source file (2024-03-25)
Supplement: Supplementary file 1 [file 99_appendix_1.tex]

\section{Feature Engineering}
% \TL{This is in simulation right?}
\label{subsec:feat_eng}
A control-variable experiment is performed to investigate the effectiveness of the feature engineering function in Section \ref{subsub:mlp} and the batch normalization block.
Figure \ref{fig:loss_evo_bn} shows that evenly distributing the features by feature engineering is the key for the network to converge.
Taking the cubic root of inputs without batch normalization is the best method which has the lowest testing loss.
Therefore, we adopt the feature engineering function $f(B) = \sqrt[3]{B}$ for all the neural networks in evaluation.

\begin{figure}
    \centering
    \includegraphics[width=1.0\linewidth]{figures/loss_evo_feat_eng.pdf}
    \caption[Testing Loss Evolution of Networks with Batch Normalization and/or Feature Engineering]{The testing loss with the identical $10^6$ random inputs per epoch fed to train networks with different input manipulations.
      \label{fig:loss_evo_bn}}
\end{figure}

\section{Algorithms}
\label{sec:algo_code}
Algorithm \ref{algo:coor_trans} is used for generating shape-specific datasets of magnetic signals, transforming $2$-dimensional signals from FEM into $3$-dimensional synthetic experimental data for training and evaluating neural networks. Definitions of variables in Algorithm \ref{algo:coor_trans} are in Table \ref{tab:var_trans}.\par
Algorithm \ref{algo:optimization} shows the implementation of optimization-based tracking used in evaluation. We add a positional judgement to prevent the results of non-converging rounds (when positional estimation is moved too far away) from impacting too much on later steps.

\begin{algorithm}[!h]
\caption{Coordinate Transformation Algorithm}\label{algo:coor_trans}
\begin{algorithmic}[1]
% \Procedure{Get Simulated Magnetic Field through Transformation Matrix}{}
\BState \textbf{Input} $\mathbf{p}^{D}_s$
\BState $\mathbf{p}_d^{D} \gets \mathbf{p}^{D}_m - \mathbf{p}^{D}_s$ \Comment Magnet-sensor vector
\BState $\mathbf{v} \gets \mathbf{w} \times \mathbf{p}_d^{D}$
\While {$\mathbf{v} = \mathbf{0}$} \Comment When $\mathbf{w}$ and $\mathbf{p}_d^{D}$ are (anti-)parallel
\State random $\mathbf{q}$
\State $\mathbf{v} \gets \mathbf{q} \times \mathbf{w}$
\EndWhile
\BState $\mathbf{u} \gets \mathbf{v} \times \mathbf{w}$
\BState $dw \gets \mathbf{p}_d^{D} \cdot \frac{\mathbf{w}}{||\mathbf{w}||}$ \Comment the projection of $\mathbf{p}_d^{D}$ on $\mathbf{w}$
\BState $du \gets \sqrt{|\mathbf{p}_d^{D}|^2 - dw^2}$ \Comment the projection of $\mathbf{p}_d^{D}$ on $\mathbf{u}$
\BState $dv \gets 0 $
\BState $\mathbf{B}^{M} \gets \mathbf{FEM}(du, dw)$
\BState \parbox[][28pt][c]{232pt}{$\mathbf{M} \gets \big[\begin{smallmatrix}
  \frac{\mathbf{u}}{||\mathbf{u}||}^\top & \frac{\mathbf{v}}{||\mathbf{v}||}^\top & \frac{\mathbf{w}}{||\mathbf{w}||}^\top \end{smallmatrix}\big]^\top $ \\ \phantom{====} \Comment Coordinate transformation matrix}
\BState $\mathbf{B}^{D} \gets \mathbf{B}^{M} \cdot \mathbf{M}$
\end{algorithmic}
\end{algorithm}

\begin{table}[h]
    \centering
        \caption[Variables in Coordinate Transformation Algorithm]{Variables notation in the coordinate transformation algorithm \ref{algo:coor_trans}.
        % \TL{Can be in appendix I think.}
        \label{tab:var_trans}}
    \begin{tabular}{ll}
    \hline
    \emph{Variables and Symbols} & \emph{Denotation}\\
    \hline
		\parbox[][16pt][c]{30pt}{$\mathbf{p}^{C}_i$} & Positional vector\\
		$C \in \{D, M\}$  & \parbox[][28pt][c]{155pt}{Positional vector is in the coordinate system of the sensor array or the magnet}\\
		$i \in \{s, m\}$ & Positional vector of a sensor or the magnet\\
		$\mathbf{u, v, w}$ & \parbox[][28pt][c]{155pt}{3 vectors aligned with the magnet's coordinate axes in $C_{D}$}\\
        $\mathbf{w}$ & \parbox[][28pt][c]{155pt}{the vector aligned with the magnetic moment vector in $C_{D}$}\\
    \hline
    \end{tabular}
\end{table}

\begin{algorithm}
\caption{Optimization-Based Method for Tracking in Simulation}\label{algo:optimization}
\begin{algorithmic}[1]
\BState Generate trajectory $\mathbf{P}_t$ and corresponding sensor reading series $\mathbf{B}$
\BState $\mathbf{p}_0 \gets$ permute($\mathbf{P}_t \lbrack 0 \rbrack$) \Comment Permute the first point as initial estimation
\BState $\mathcal{S} \gets$ interactive space
\For {$i = 0, \ldots, n-1$ }
    \State $\mathbf{p}_i^\prime \gets $ optimize($\mathbf{p}_i, \mathbf{B}_i$)
    \If {$\mathbf{p}_i^\prime \in \mathcal{S}$} \State $\mathbf{p}_{i+1} \gets \mathbf{p}_i^\prime$
    \Else \State $\mathbf{p}_{i+1} \gets \mathbf{p}_i$
    \EndIf
\EndFor
\end{algorithmic}
\end{algorithm}
